# Supplementary material for: Graph Embedded Pose Clustering for Anomaly Detection
Source: arXiv:1912.11850 source file (2020-04-10)
Supplement: Supplementary file 1 [file appendix.tex]

\clearpage
{\small
\bibliographystyle{ieee}
\bibliography{egbib}
}
\input{supp_files/kinetics250_class_list.tex}
