# Supplementary material for: Graph Embedded Pose Clustering for Anomaly Detection
Source: arXiv:1912.11850 source file (2020-04-10)
Supplement: Supplementary file 2 [file fail_cases_kin_para.tex]

\section{Fail Cases - \emph{Kinetics-250}} \label{supp_kin_fail_cases}
Figure~\ref{fig:fail_cases} shows some failure cases. The recovered pose graph is super-imposed on the image. As can be seen, there is significant variability in scenes, viewpoints and poses of the people in what is considered a single ``normal'' data split. The two failures depicted show the weakness on relying solely on extracted pose for representing the action in a clip. We chose failure cases in which the pose is adequately extracted so we could focus on the model itself. 
% Clearly, a failure to extract poses would harm the method's results. 
% \amir{maybe move this failure cases to supp if we don't have enough space in the main body?}

Depicted in Figure~\ref{fig:fail_cases}, a ``lunge'' class clip which is to be considered normal is labeled abnormal when the instructor performs a single, slow and mostly static lunge throughout the clip, which we assume breaks the repetitive nature associated with lunge clips. The Second case, in which a standing-up Tai-chi instructor moves his hands forward and backward in a manner that may considered to be similar to a push ups arm movement, considered ``normal'' for that split.

\begin{figure}
\begin{center}
\begin{tabular}{@{\hskip 0in}c@{\hskip 0.05in}c@{\hskip 0.05in}c@{\hskip 0.06in}@{\hskip 0in}}
\includegraphics[width=0.3\linewidth]{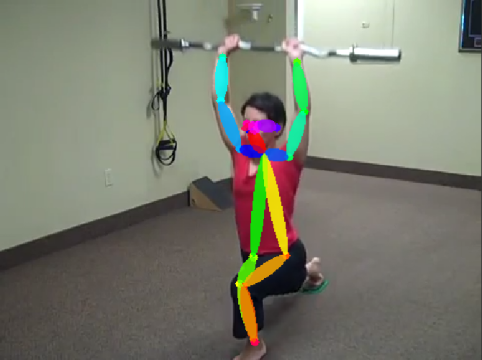} & 
\includegraphics[width=0.3\linewidth]{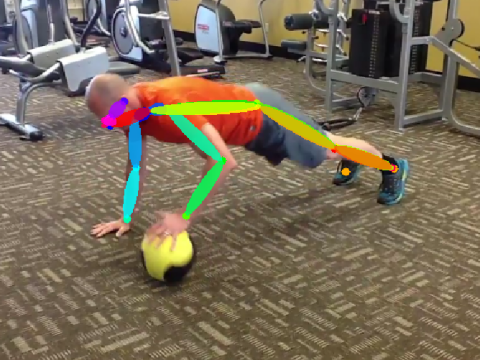}  &
\includegraphics[width=0.3\linewidth]{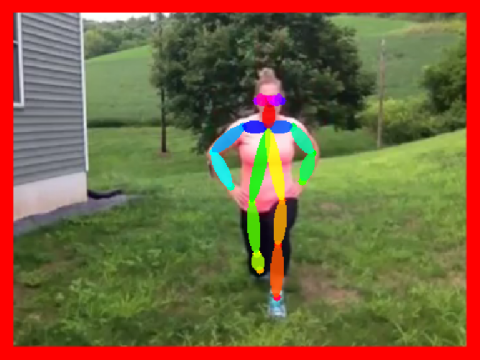} \\ 
\includegraphics[width=0.3\linewidth]{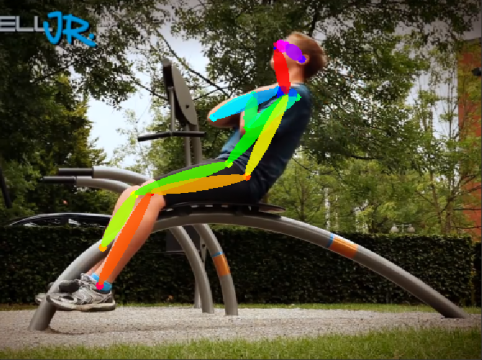} & 
\includegraphics[width=0.3\linewidth]{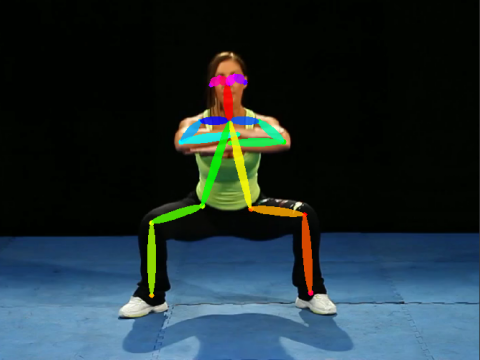} & 
\includegraphics[width=0.3\linewidth]{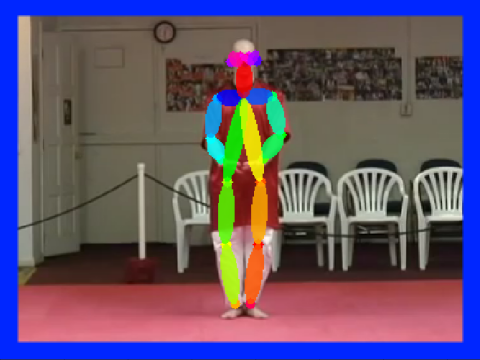} \\

\multicolumn{1}{c}{(a)} & \multicolumn{1}{c}{(b)} & \multicolumn{1}{c}{(c)}  \vspace{-0.25cm}\\
% (a) & (b) & (c) \vspace{-0.30cm}
\end{tabular}
\end{center}
\caption{{\small \textbf{Failure Cases, \textit{Kinetics-250}:} Frames overlayed with extracted poses from ``Gym'' split: Columns (a)-(b) depict dataset classes ``Lunge'', ``Push ups'', ``Situp'' and ``Squat''. Column (c) depicts failure cases; Top: a ``normal'' {\it lunge} sequence, mislabeled as ``abnormal'' in a clip where the instructor remains static for most of the time. Bottom: an ``abnormal'' {\it Tai-chi} clip labeled ``normal'' when the instructor demonstrates a push up like hand movement.}
\vspace{-0.2cm}}
\label{fig:fail_cases}
\end{figure}
