# Supplementary material for: Graph Embedded Pose Clustering for Anomaly Detection
Source: arXiv:1912.11850 source file (2020-04-10)
Supplement: Supplementary file 3 [file kinetics_roc2.tex]

\begin{figure*}
\begin{center}
\hspace*{-0.5cm}\begin{tabular}{@{\hskip 0.0cm}c@{\hskip -0.0cm}c@{\hskip -0.0cm}c@{\hskip -0.0cm}c@{\hskip 0.0cm}}
\includegraphics[width=0.41\linewidth]{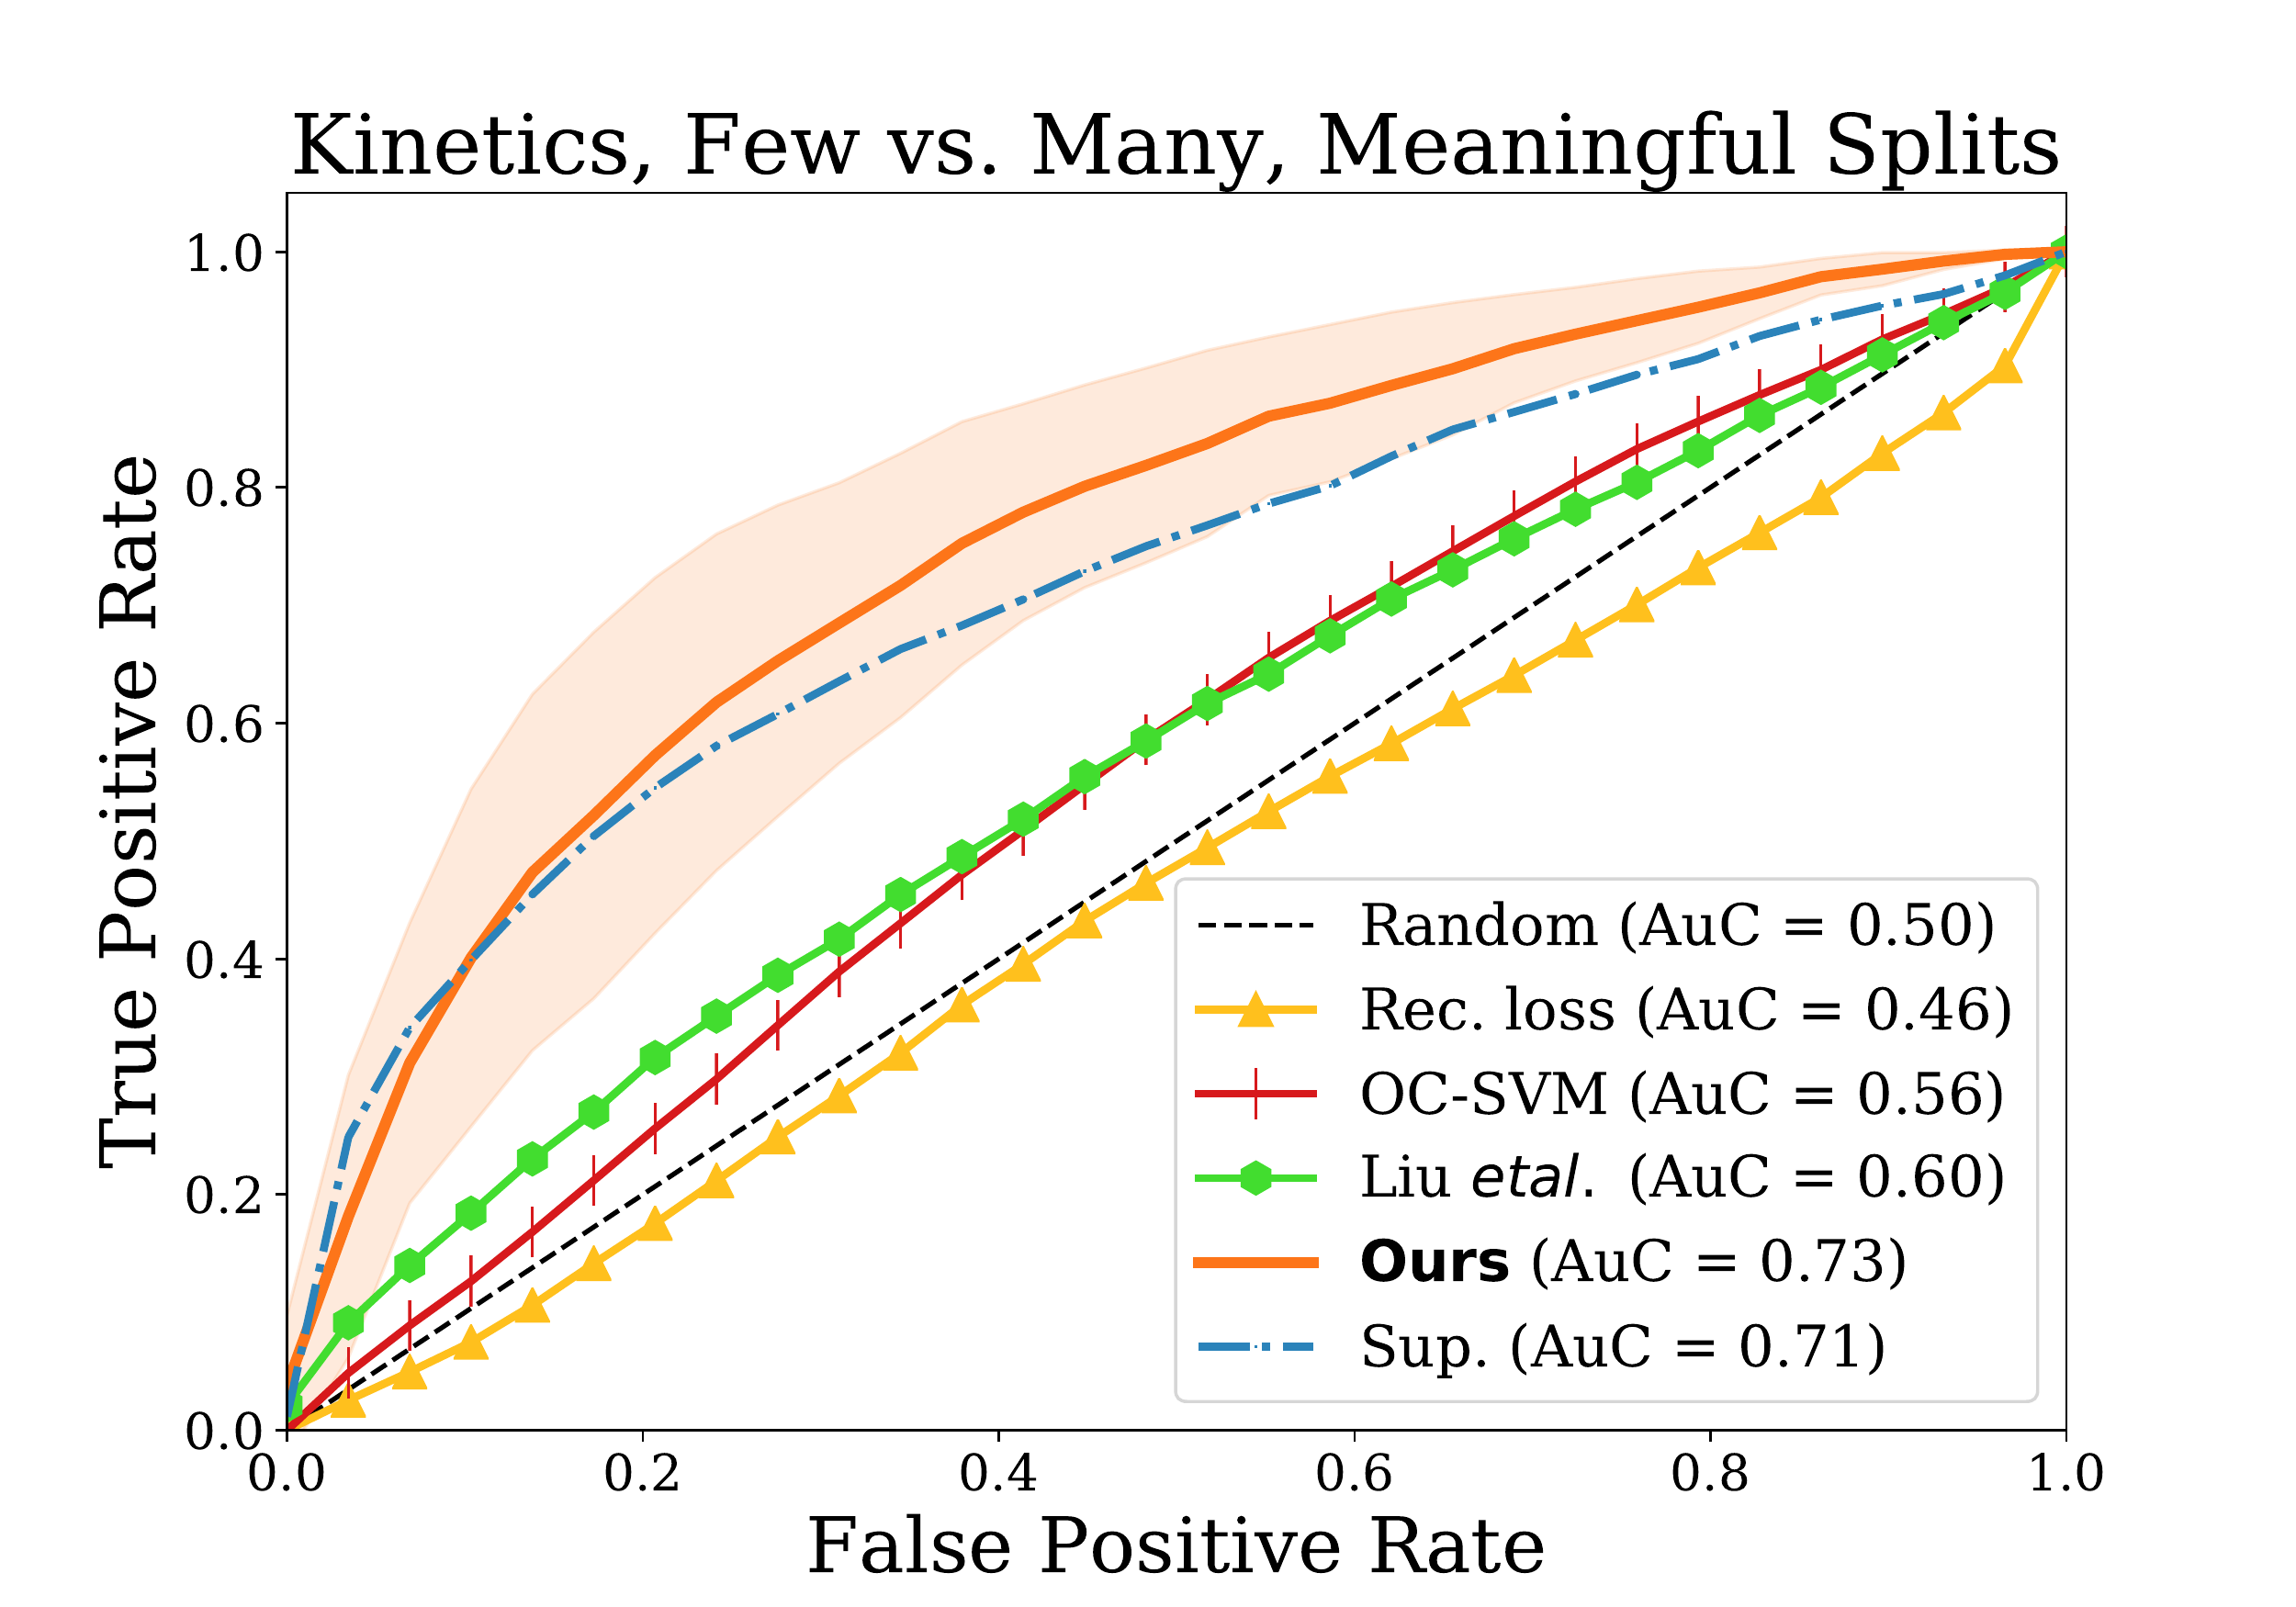} & 
\includegraphics[width=0.41\linewidth]{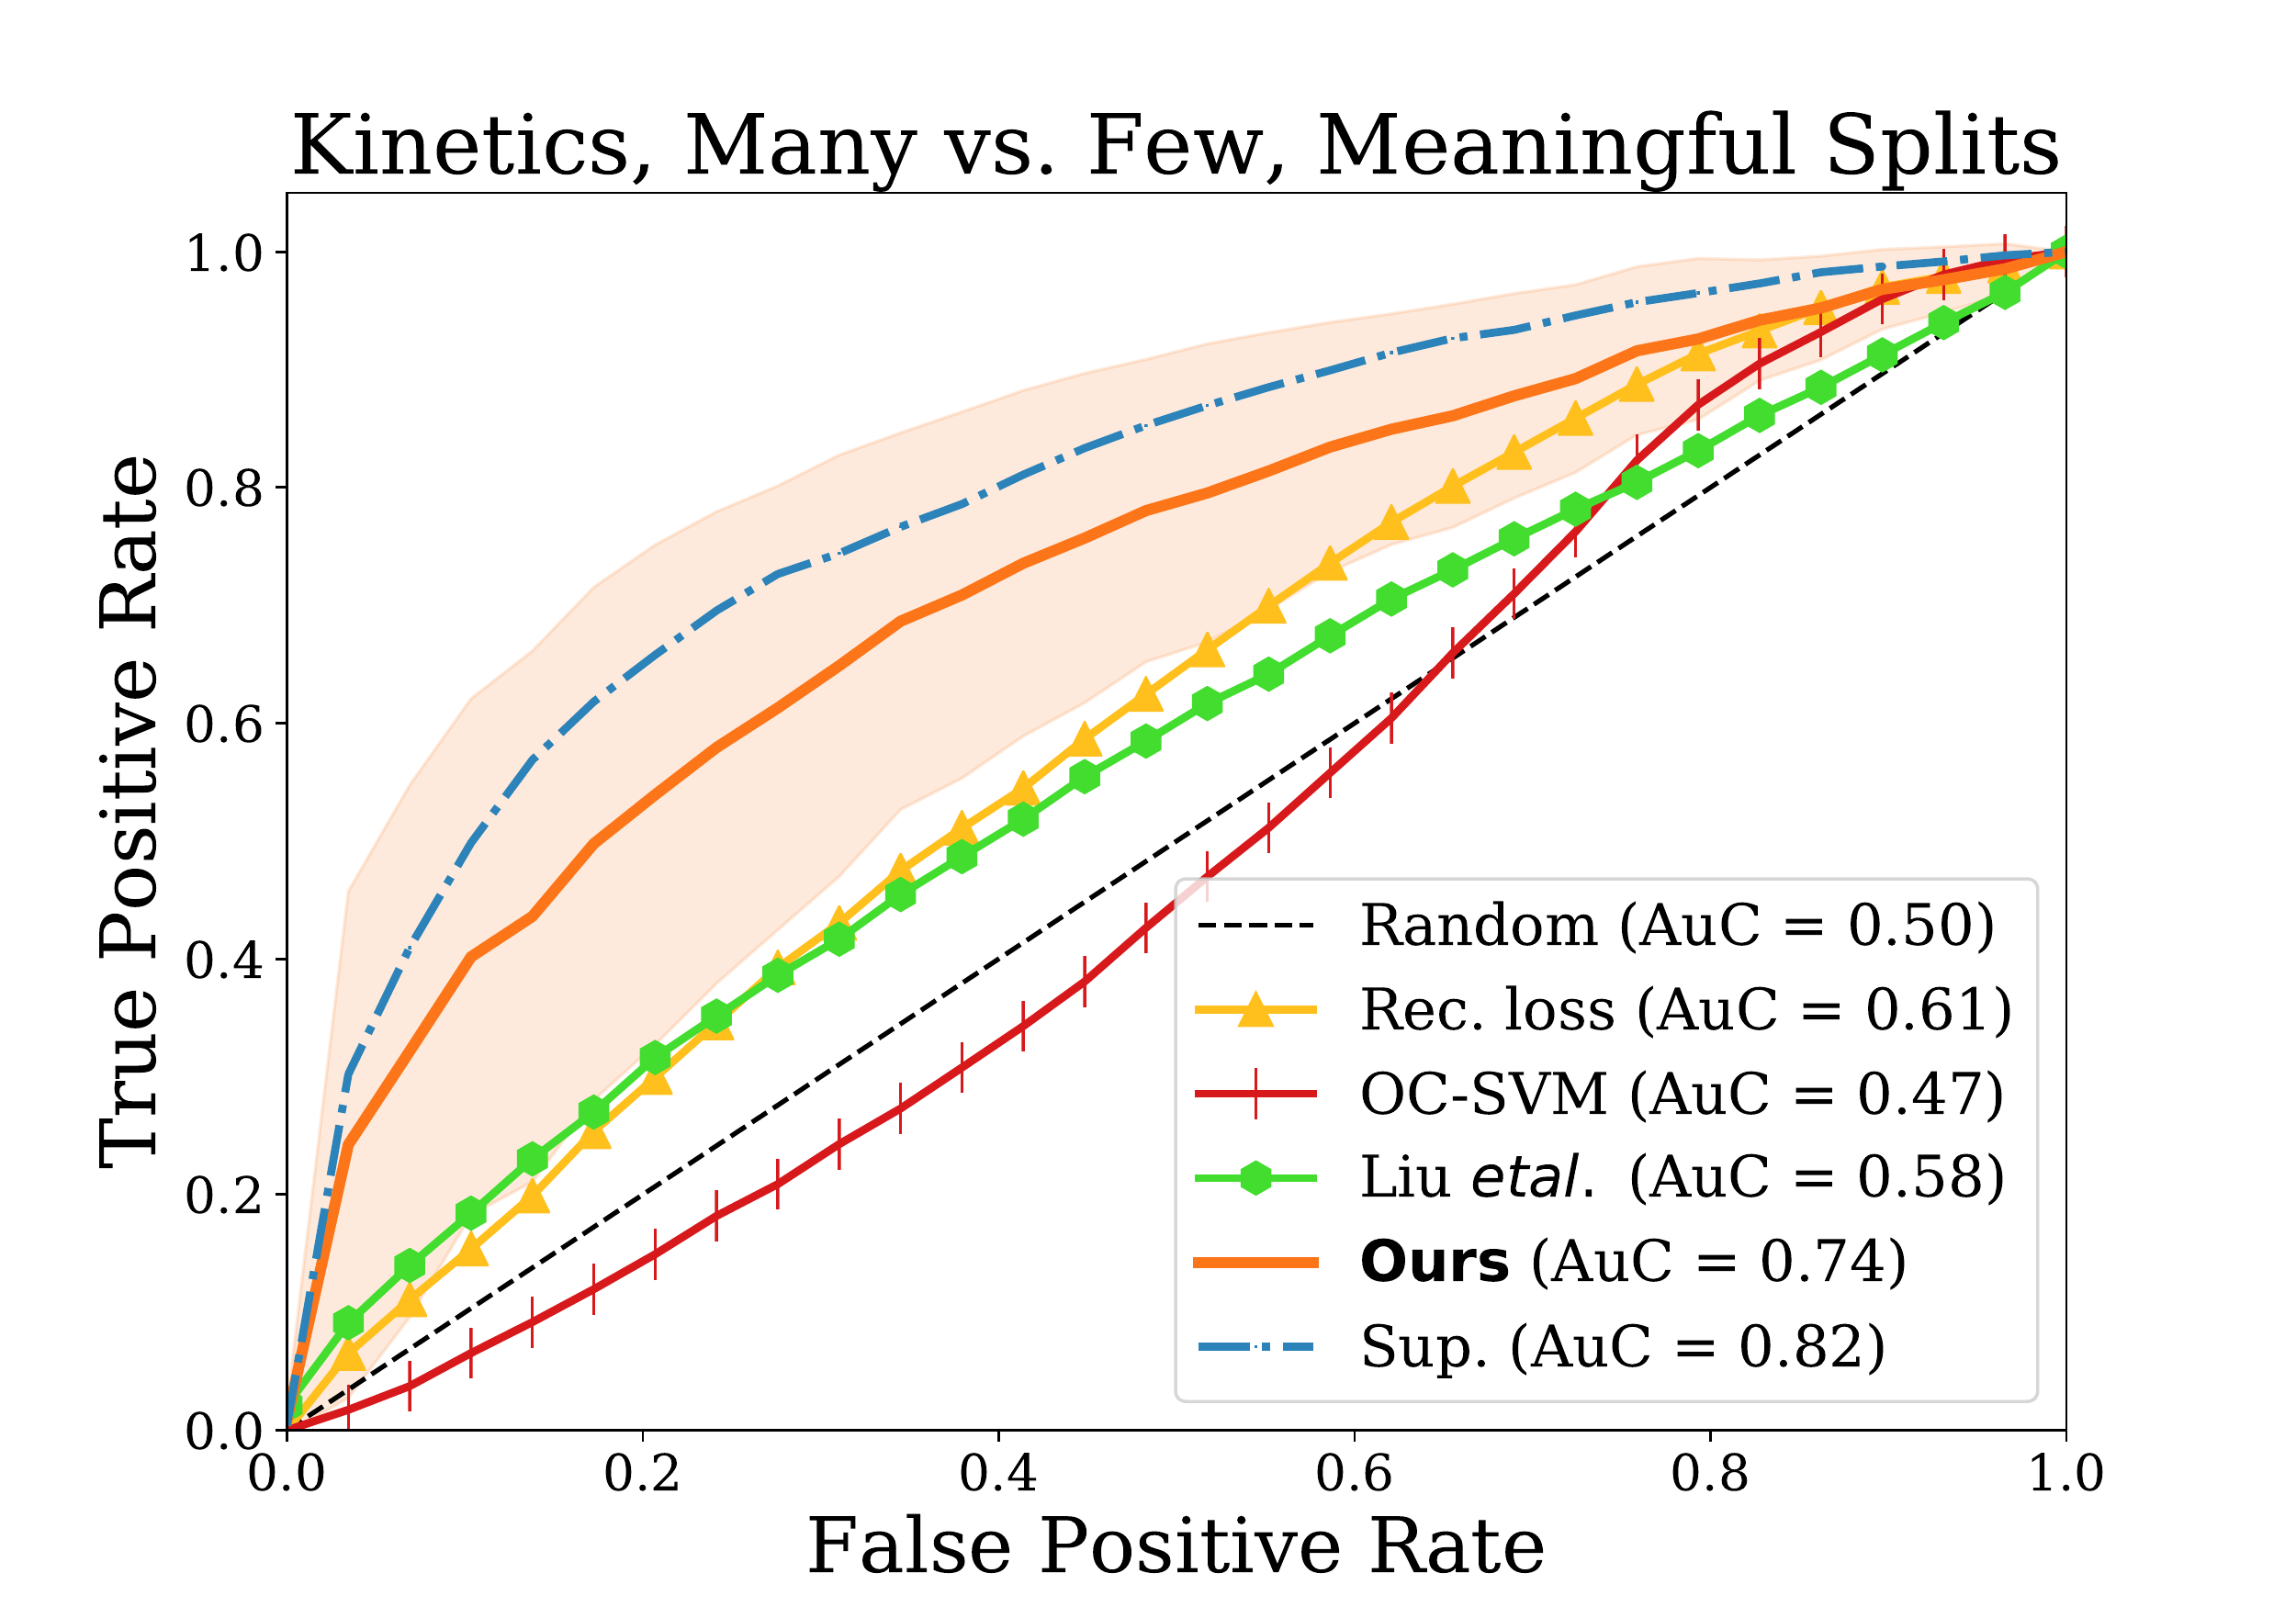} & \vspace{-0.47cm} \\
\includegraphics[width=0.41\linewidth]{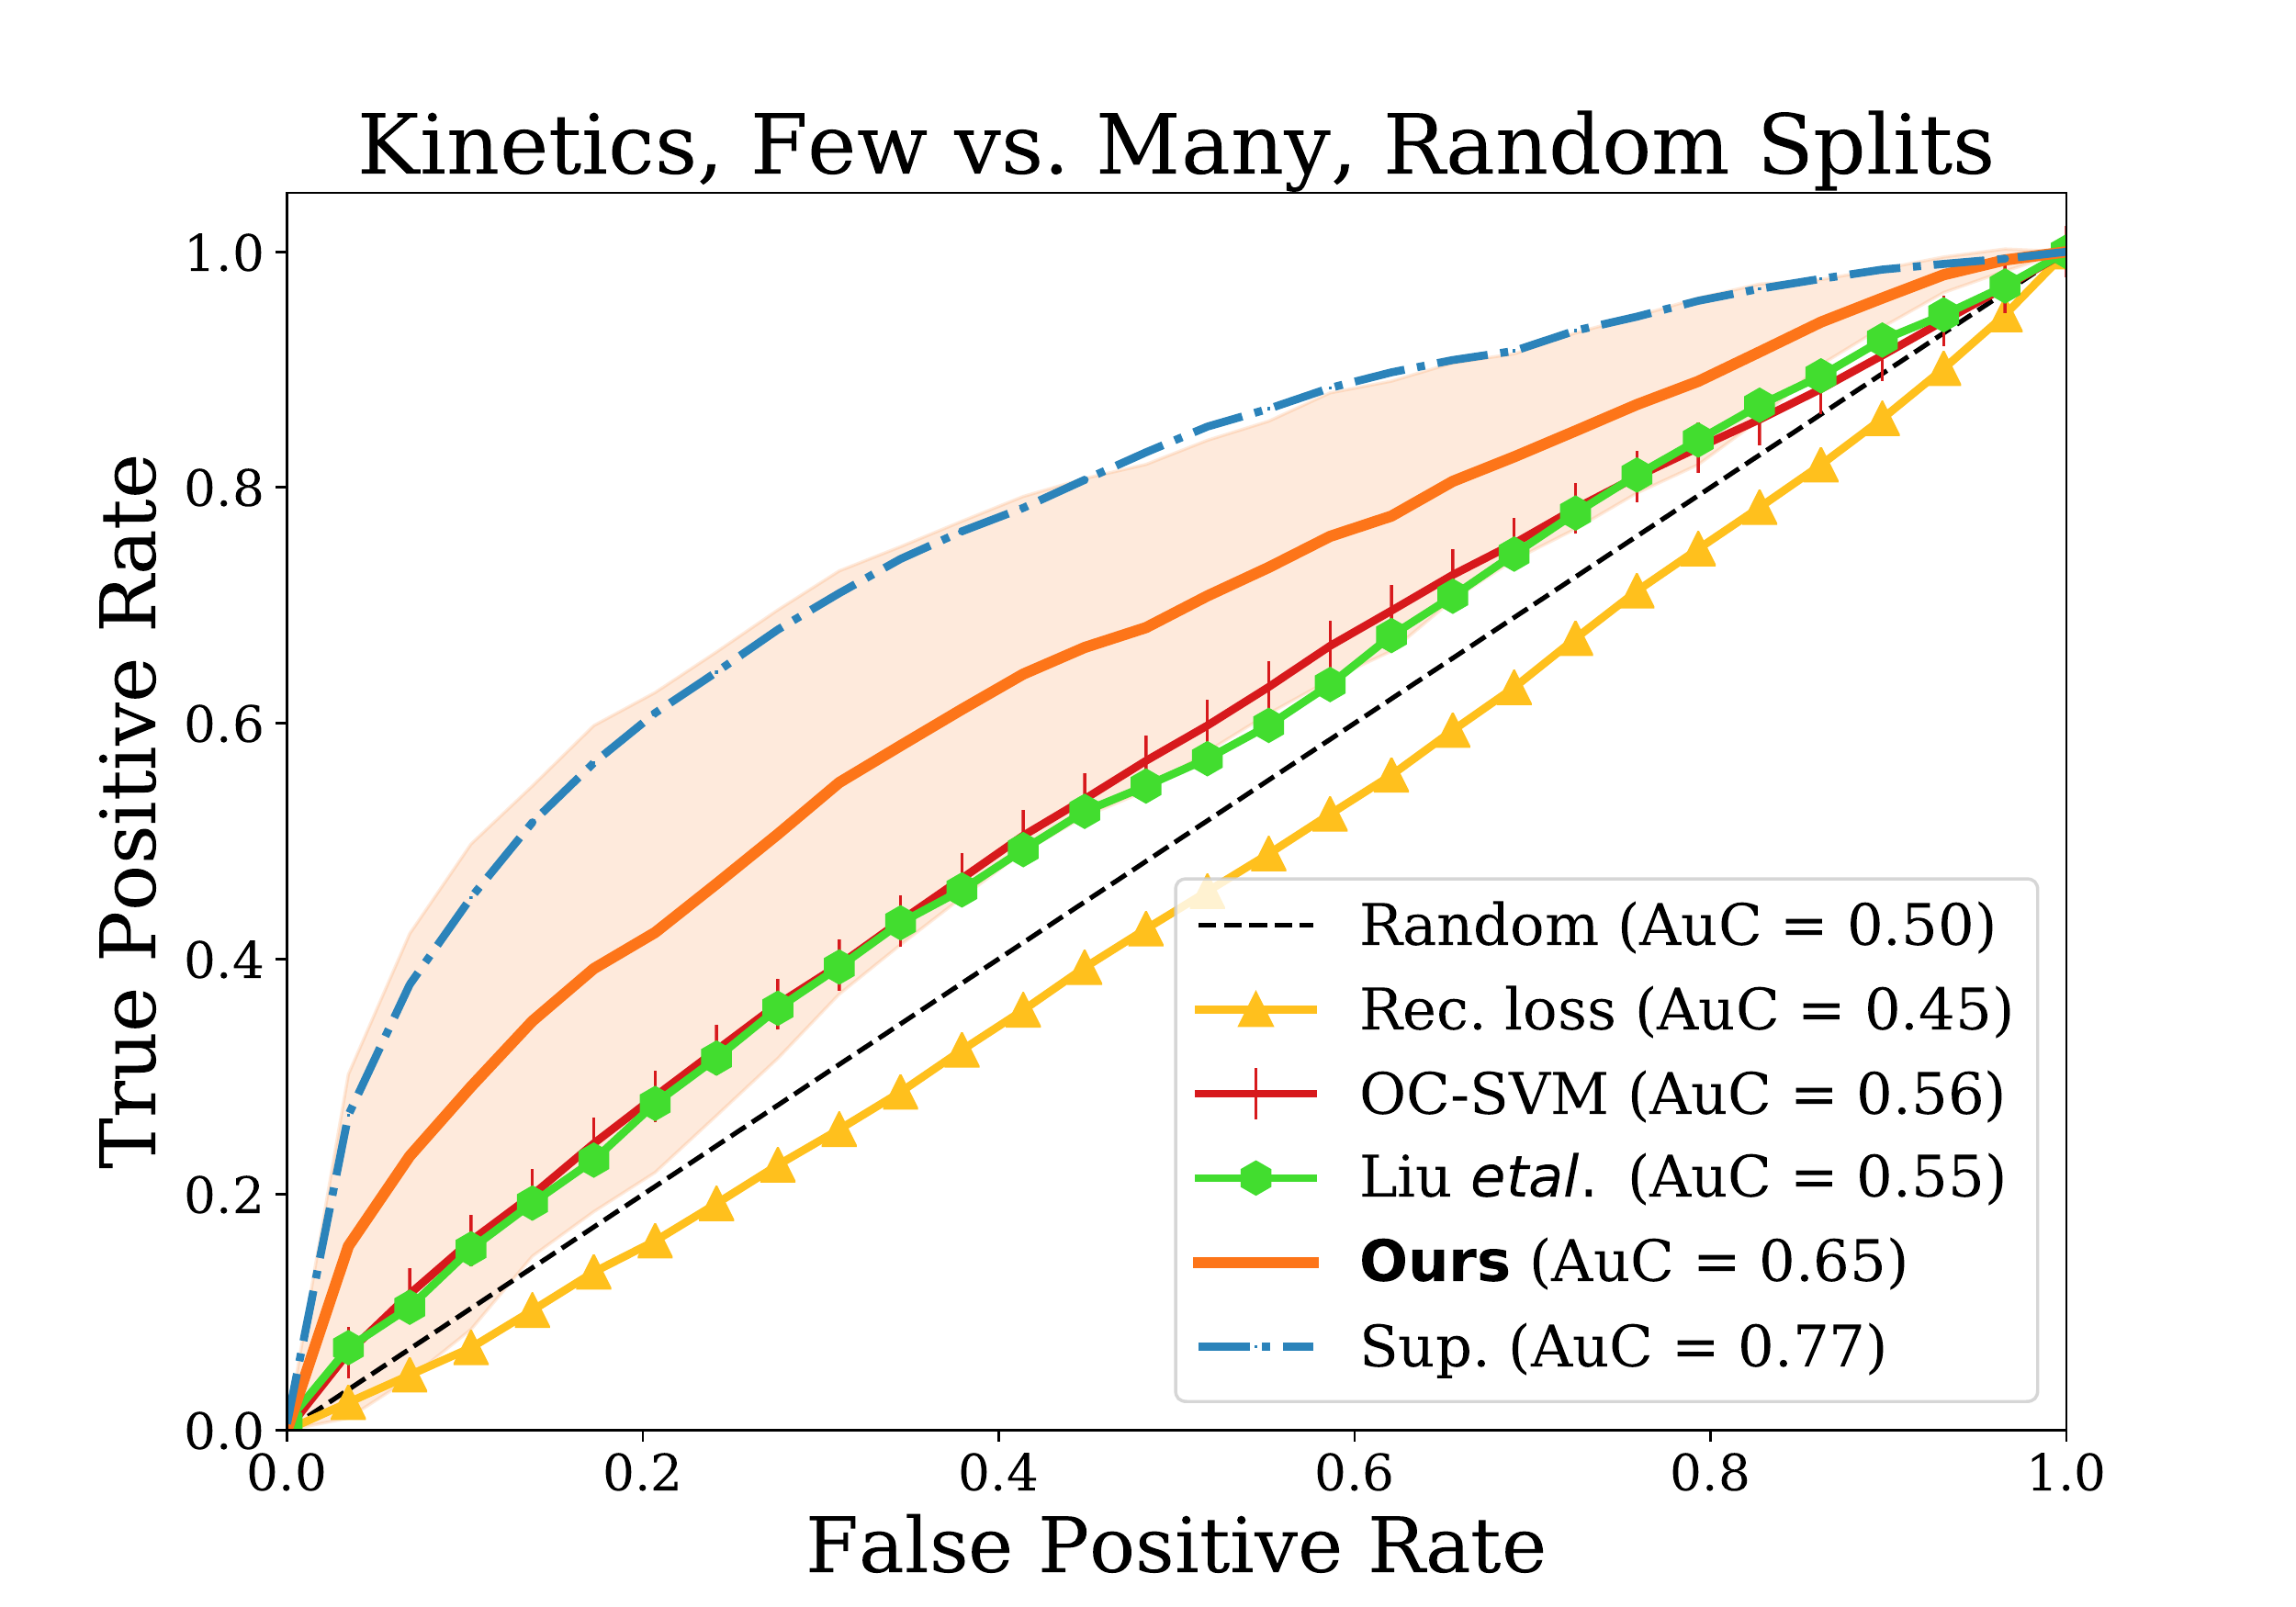} &  
\includegraphics[width=0.41\linewidth]{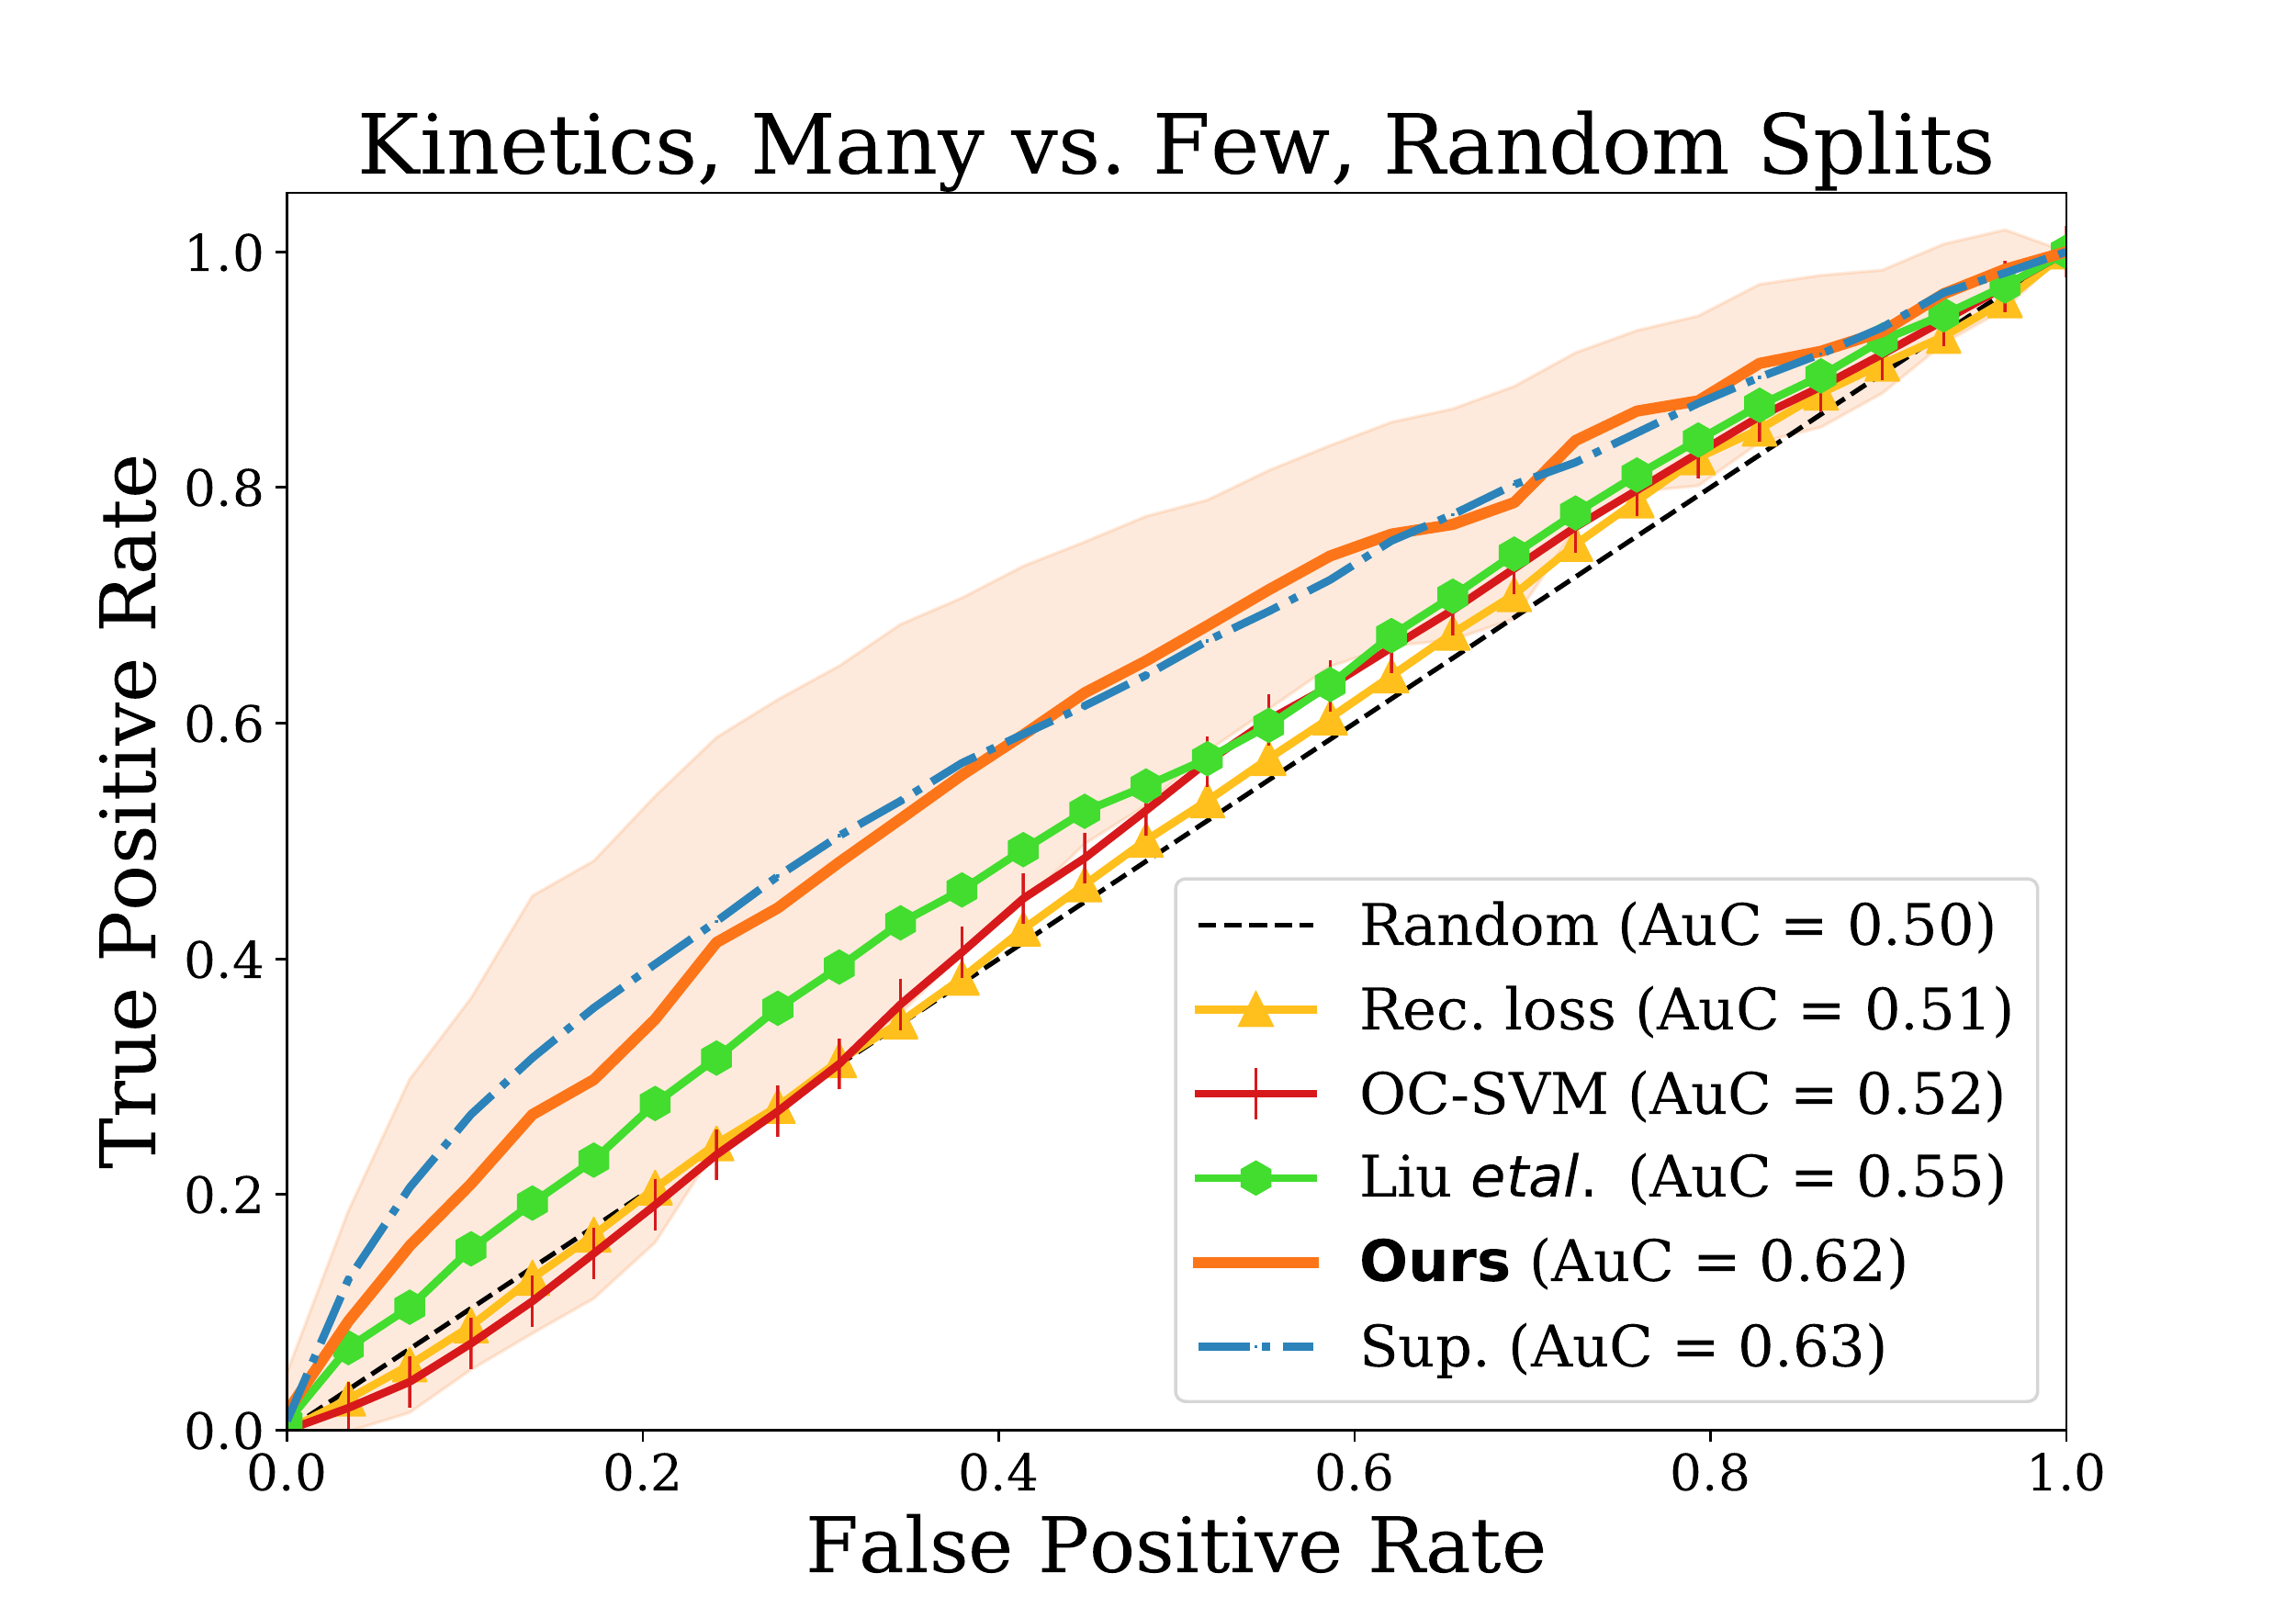}  \vspace{-0.12cm}\\
% \hspace{0.2cm}(a) & \hspace{0.2cm}(b) & \hspace{0.2cm}(c) & \hspace{0.2cm}(d) \vspace{-0.20cm}
\end{tabular}
\end{center}
\caption{{\small \textbf{Average ROC Curves for \textit{Kinetics-250} dataset.} \emph{``Sup.''} denotes the supervised baseline. Fill denotes standard deviation.}}
\label{plot:kinetics_roc}
\end{figure*}
