# Supplementary material for: Graph Embedded Pose Clustering for Anomaly Detection
Source: arXiv:1912.11850 source file (2020-04-10)
Supplement: Supplementary file 4 [file ntu_roc.tex]

\begin{figure*}
\begin{center}
% \hspace*{-0.5cm}\begin{tabular}{@{\hskip 0.0cm}c@{\hskip -0.0cm}c@{\hskip -0.0cm}c@{\hskip -0.0cm}c@{\hskip 0.0cm}}
\hspace*{-0.5cm}\begin{tabular}{@{\hskip 0.0cm}c@{\hskip -0.0cm}c@{\hskip 0.0cm}}
\includegraphics[width=0.41\linewidth]{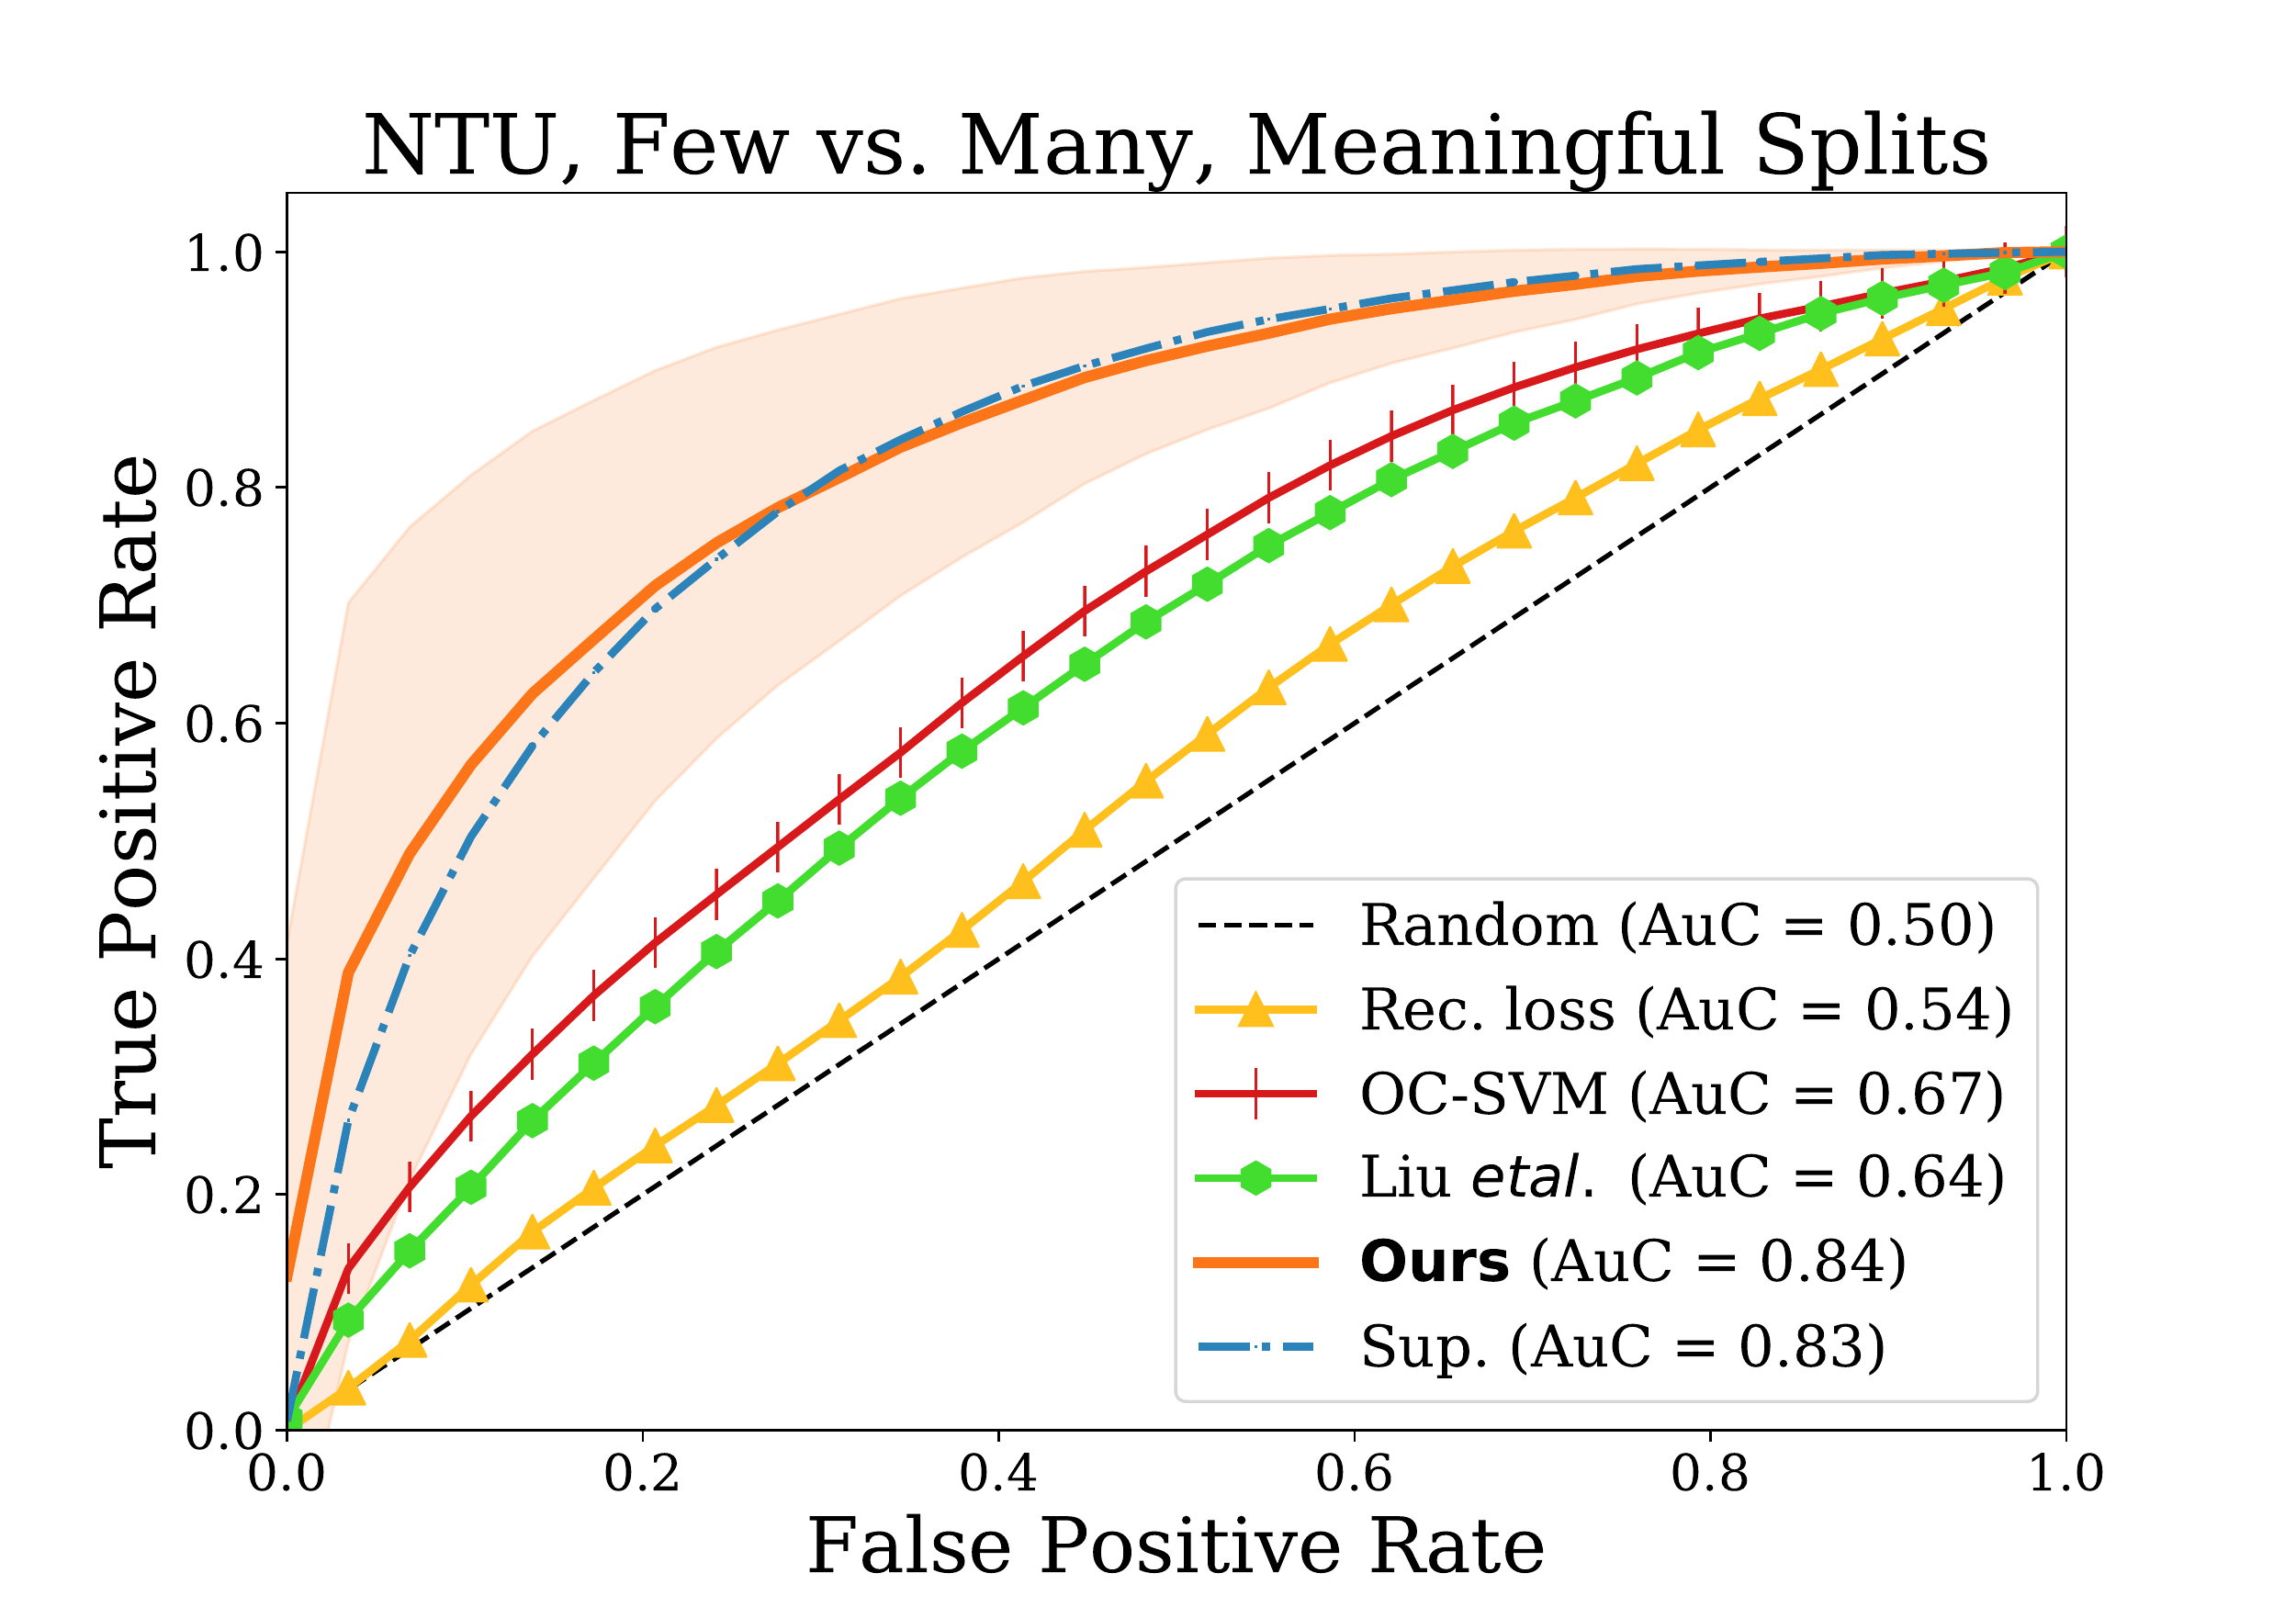} & 
\includegraphics[width=0.41\linewidth]{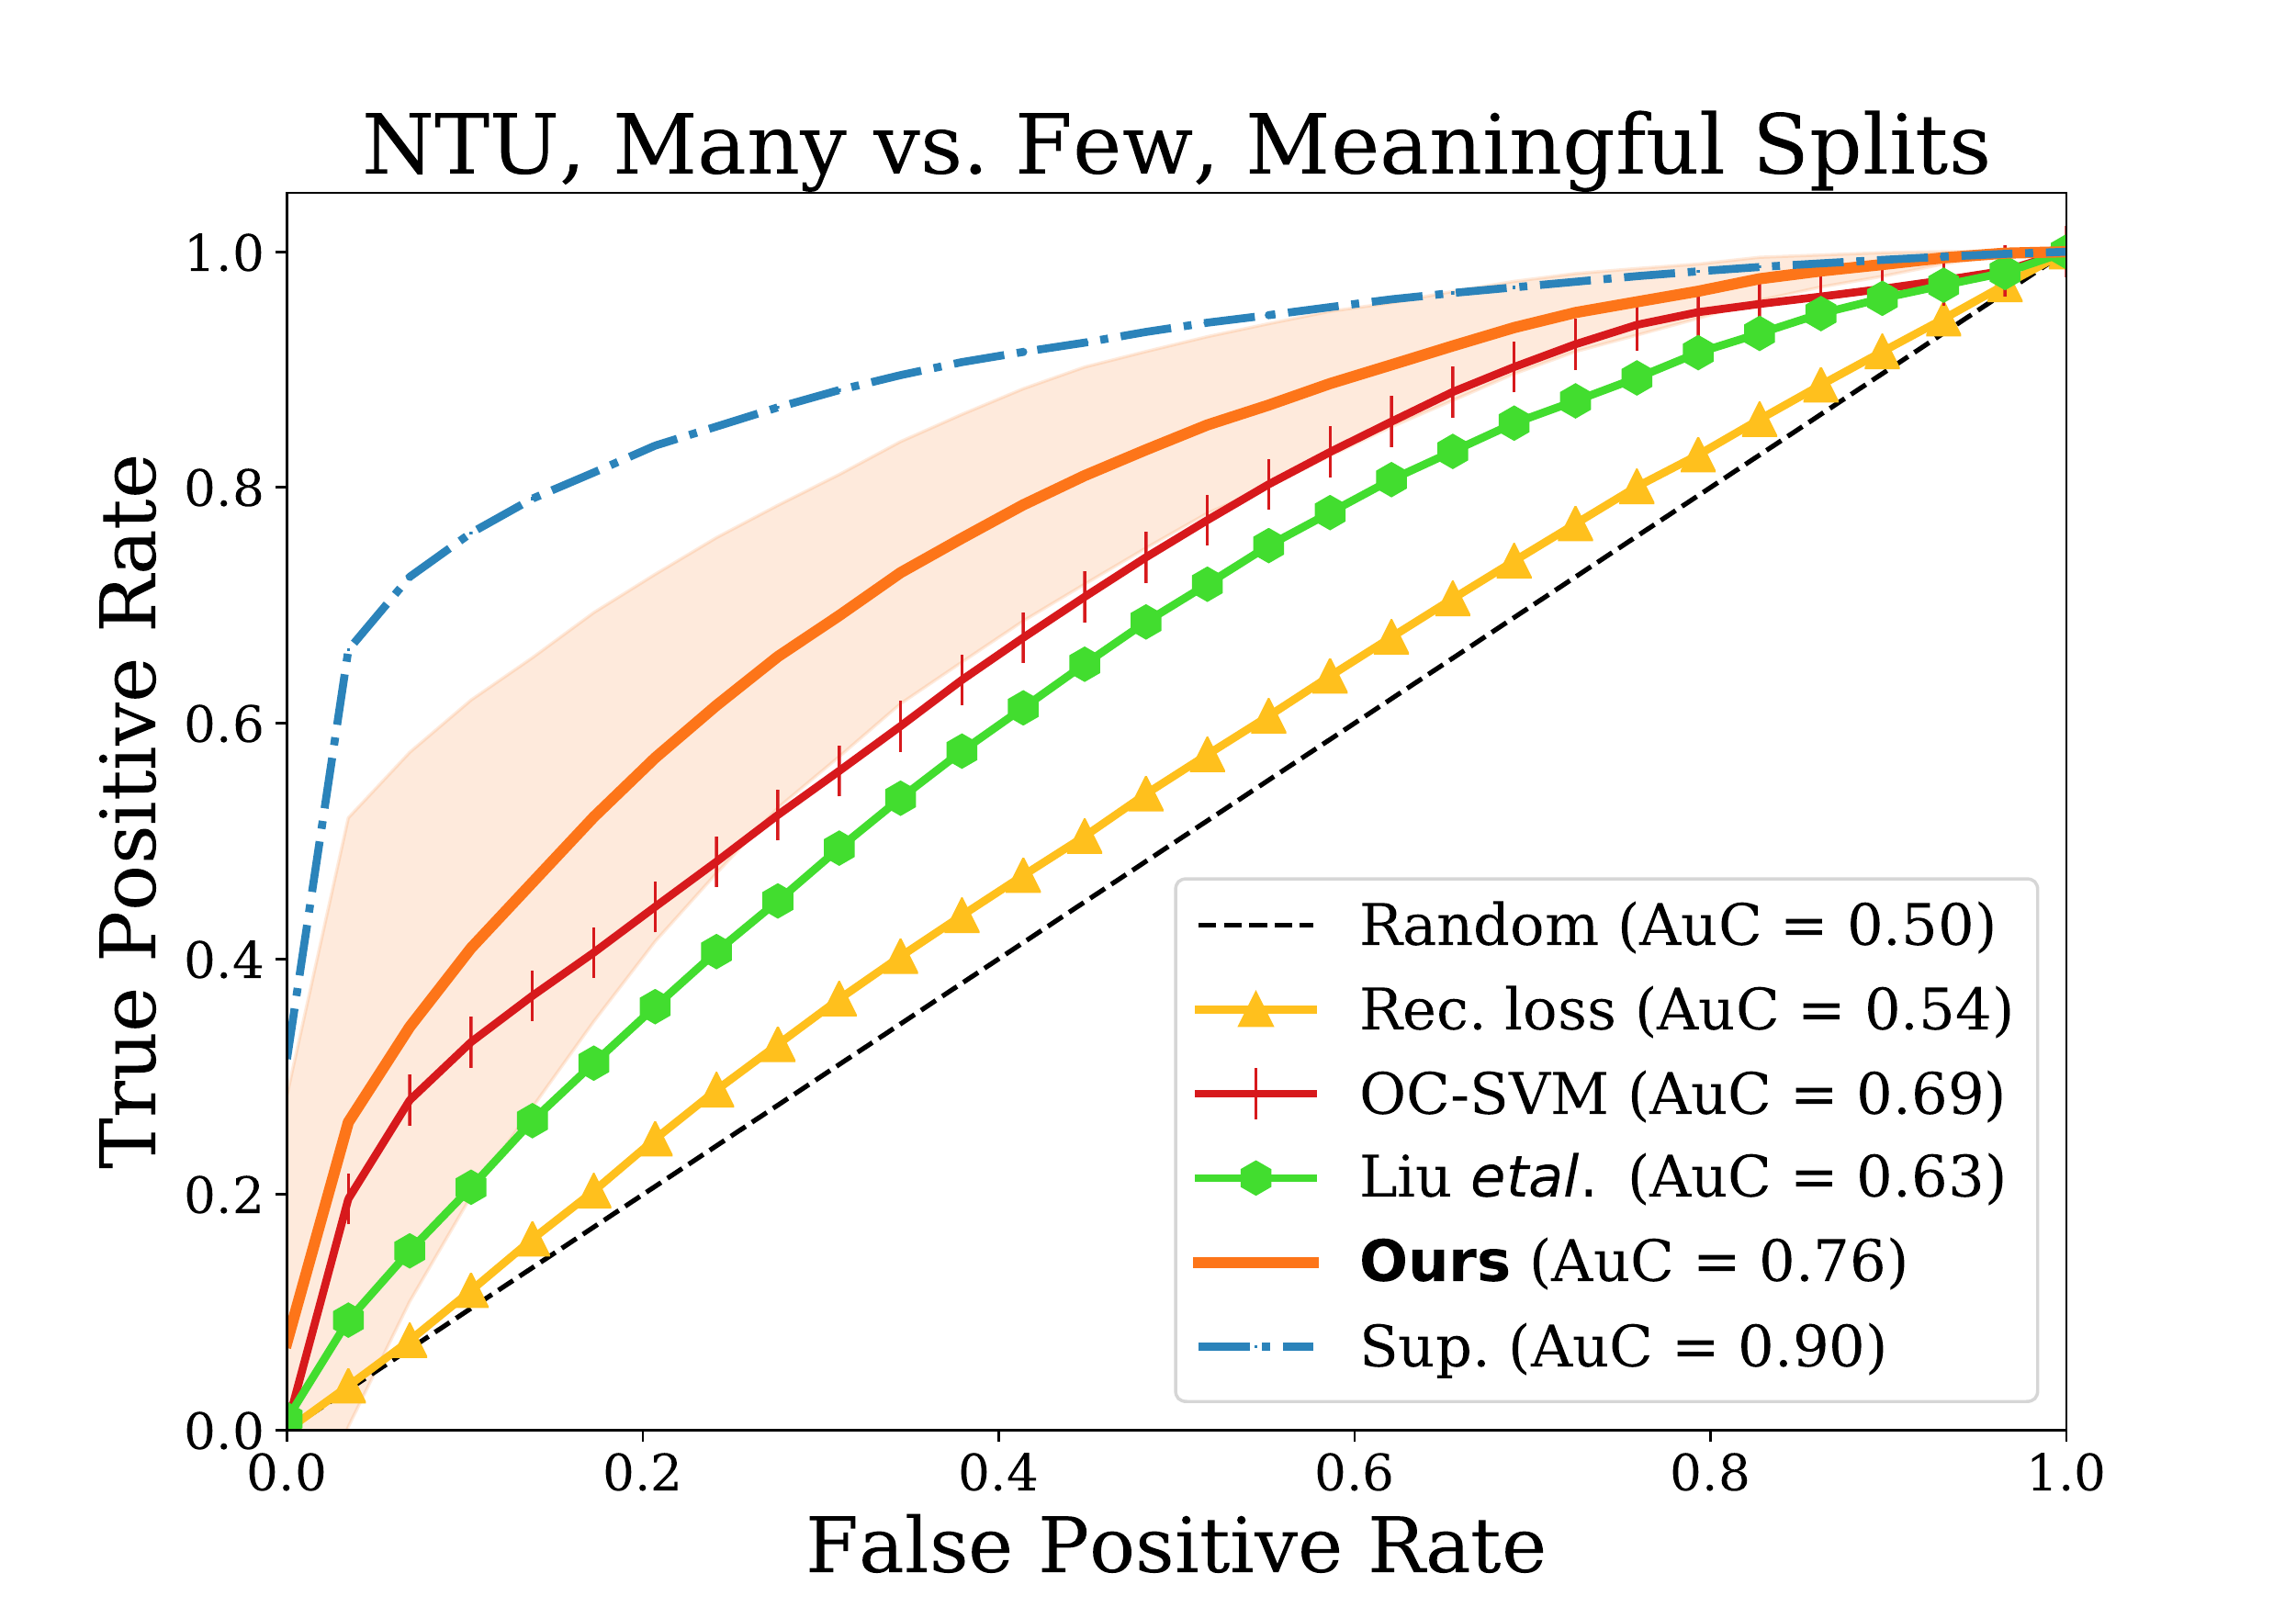} & \vspace{-0.55cm} \\
\includegraphics[width=0.41\linewidth]{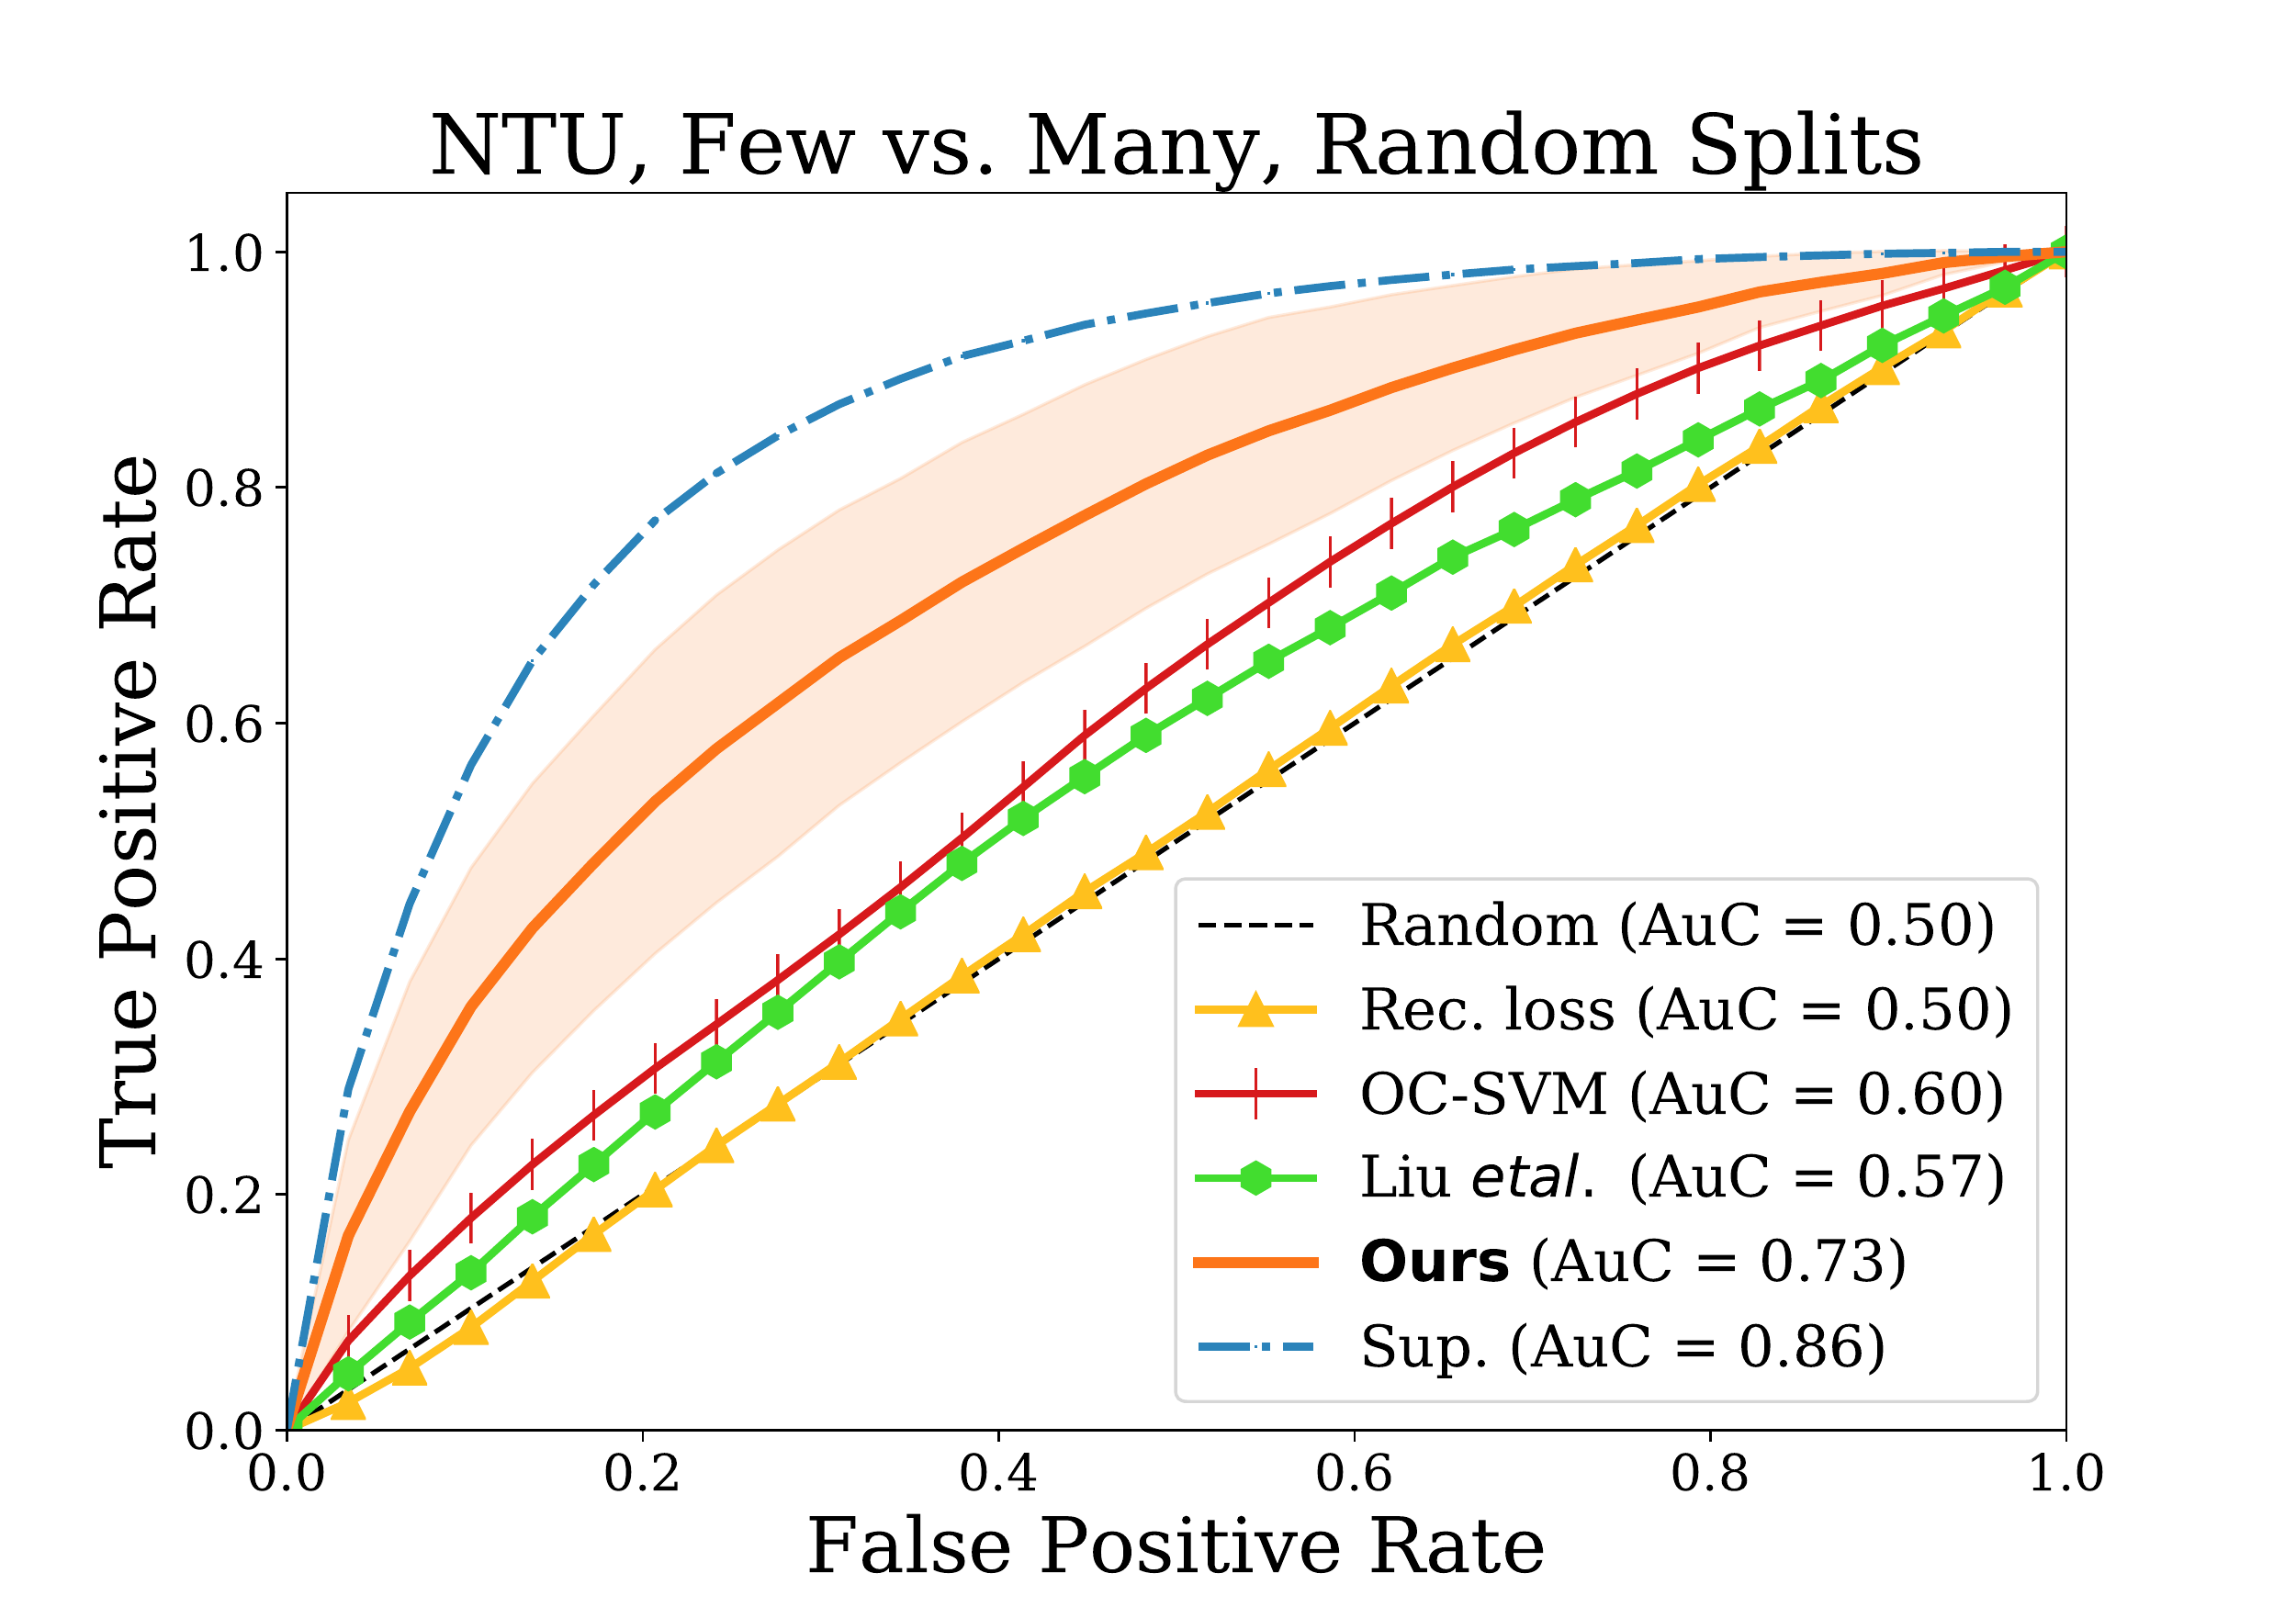} & 
\includegraphics[width=0.41\linewidth]{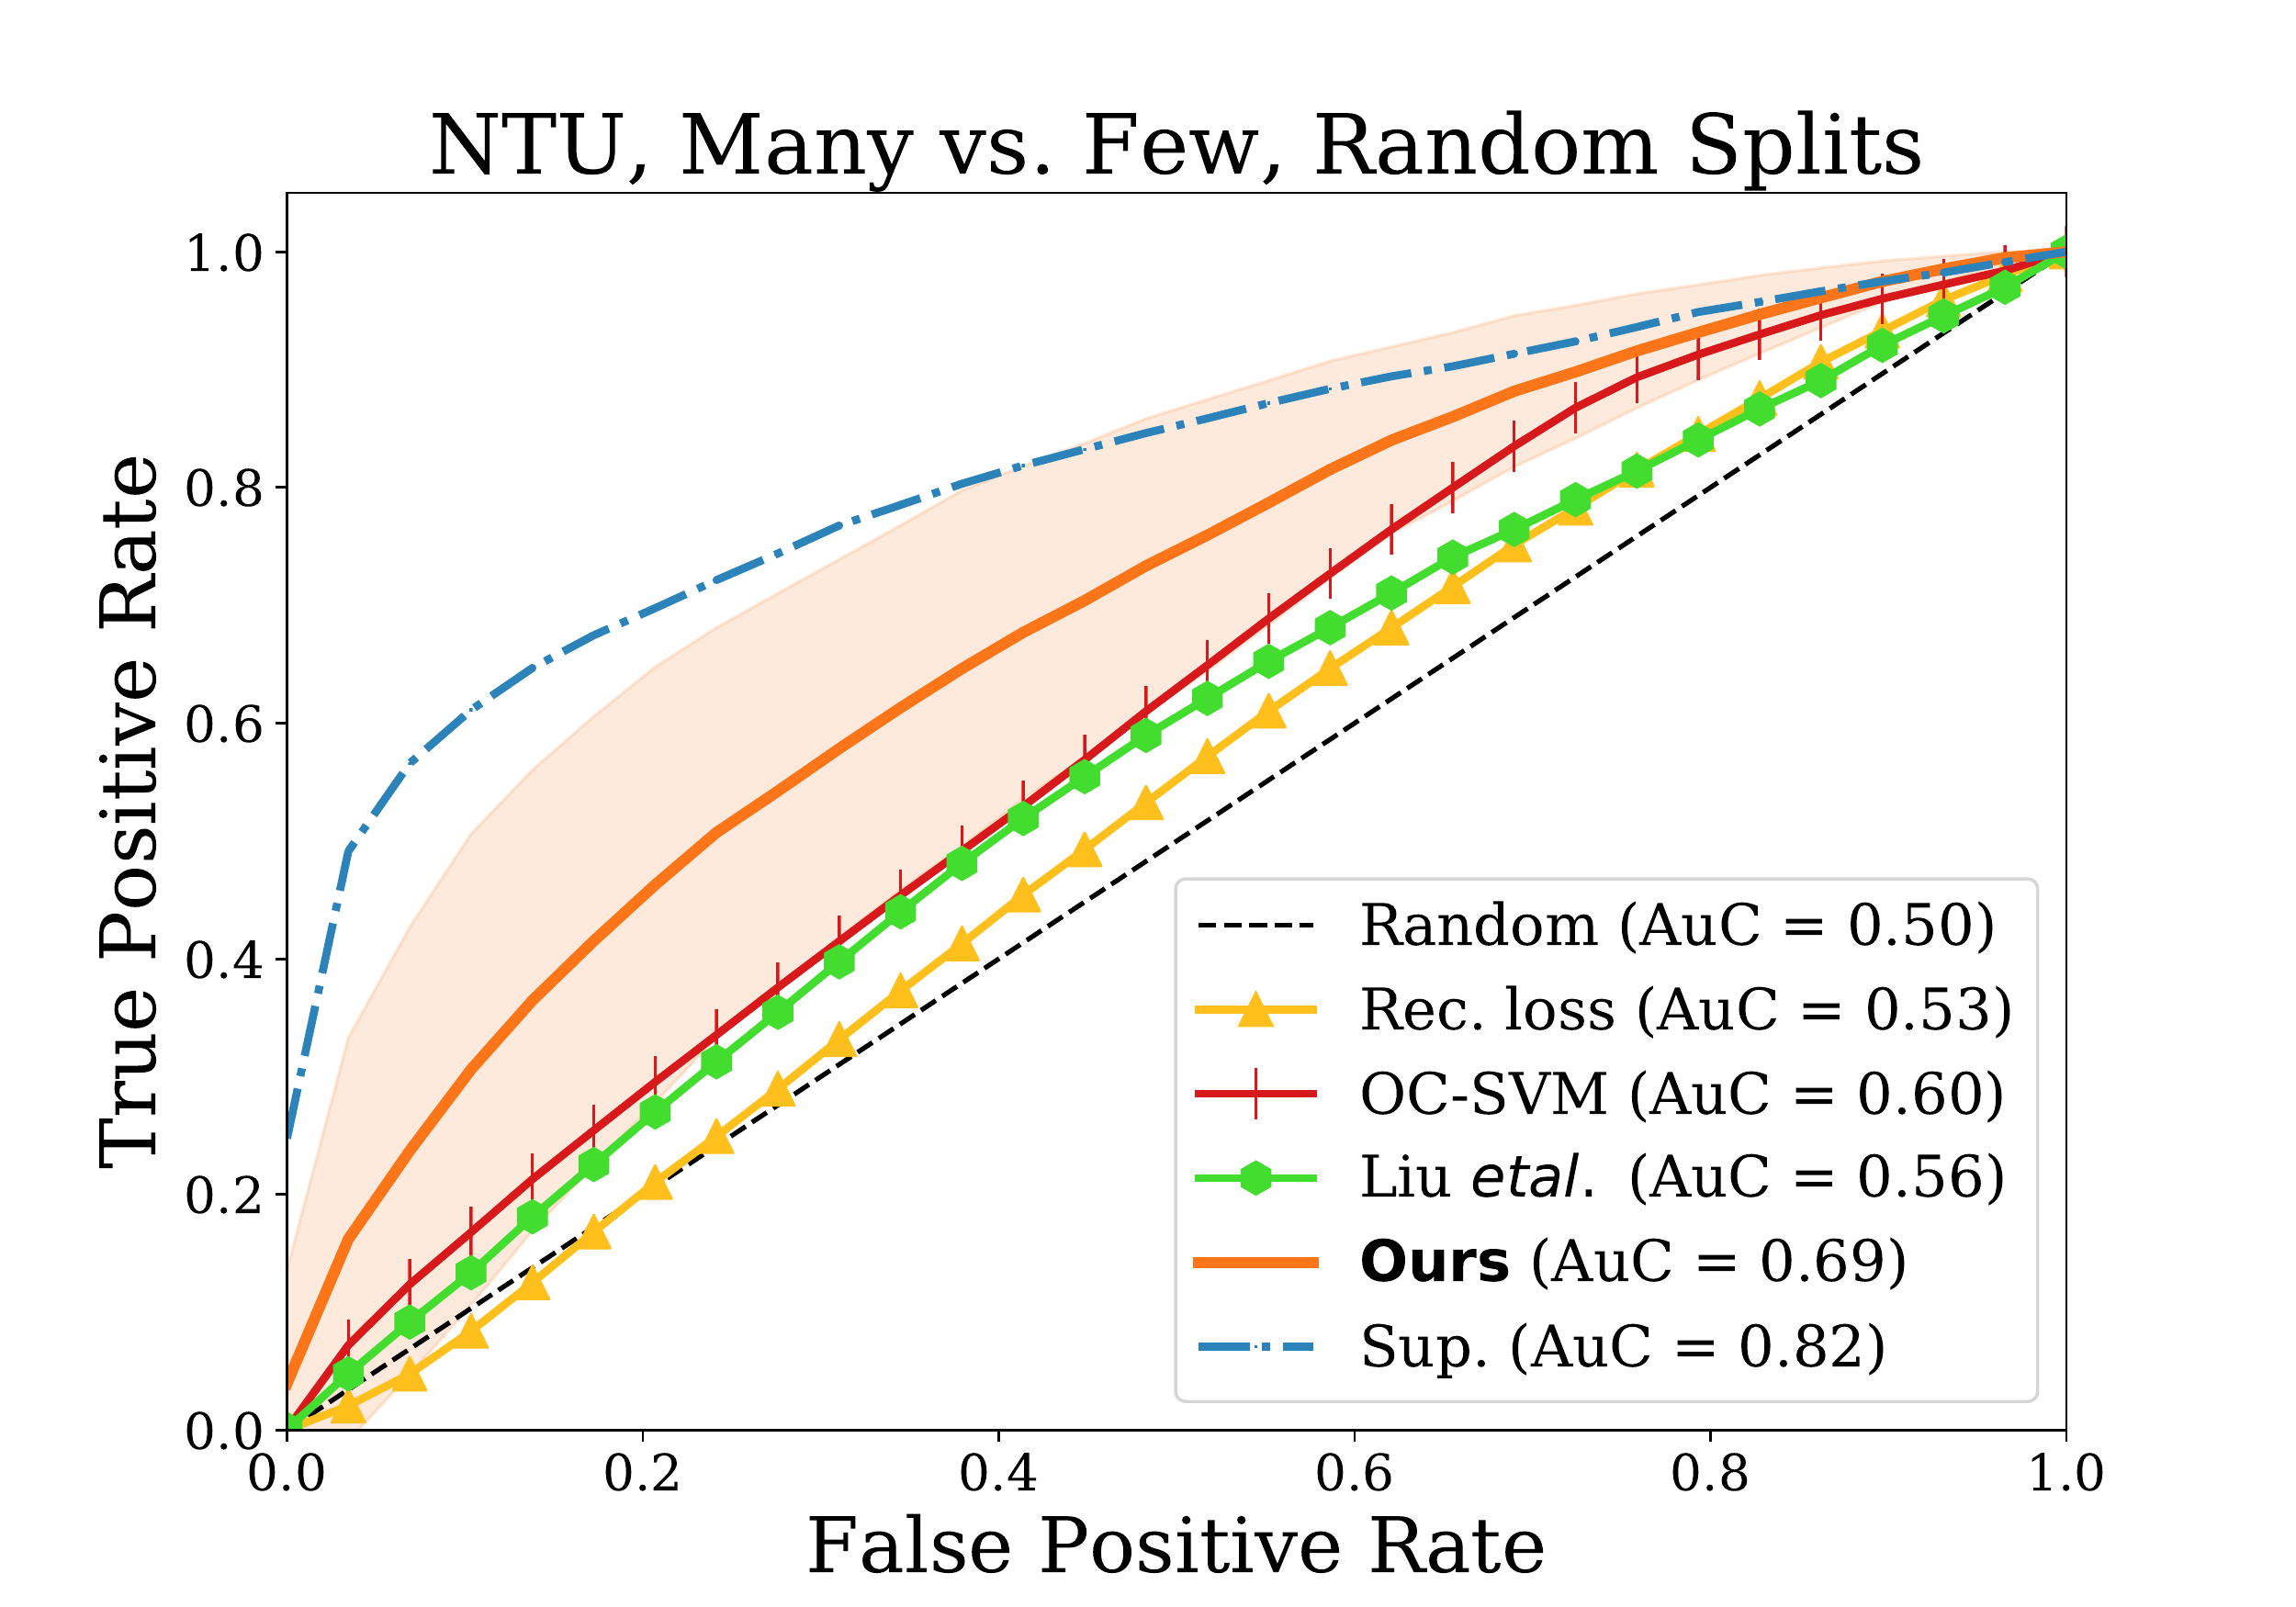}  \vspace{-0.12cm}\\
\end{tabular}
\end{center}
\caption{{\small \textbf{Average ROC Curves for \textit{NTU-RGB-D} dataset.} \emph{``Sup.''} denotes the supervised baseline. Fill denotes standard deviation. }}
\label{plot:ntu_roc}
\end{figure*}
