# Supplementary material for: Graph Embedded Pose Clustering for Anomaly Detection
Source: arXiv:1912.11850 source file (2020-04-10)
Supplement: Supplementary file 5 [file roc_figs.tex]

\section{Experiment Average ROC Curves}
The following figures depict the average ROC curves for each method for each of the settings. 
