# Supplementary material for: Graph Embedded Pose Clustering for Anomaly Detection
Source: arXiv:1912.11850 source file (2020-04-10)
Supplement: Supplementary file 7 [file basewords_fine.tex]

\begin{figure}
\begin{center}
\begin{tabular}{@{\hskip 0in}c@{\hskip 0.05in}c@{\hskip 0.05in}c@{\hskip 0.06in}@{\hskip 0in}}
\includegraphics[width=0.3\linewidth]{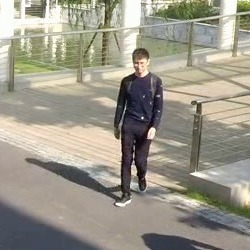} & 
\includegraphics[width=0.3\linewidth]{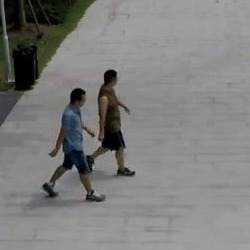} & 
\includegraphics[width=0.3\linewidth]{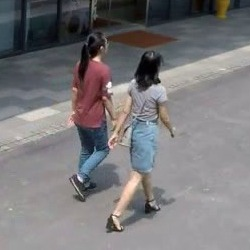} \\

\multicolumn{1}{c}{(a)} & \multicolumn{1}{c}{(b)} & \multicolumn{1}{c}{(c)} \\ % \vspace{-0.15cm}\\

\end{tabular}
\end{center}
\caption{
{\small 
\textbf{Base Words, \textit{Fine-grained}:} 
Samples closest to cluster centroids, from a model trained on \emph{ShanghaiTech} dataset. Frames from clips whose cluster assignment is closest to hard-assignment (one-hot), from three different clusters. 
Column (a) depicts a person walking towards the camera;
Column (b) depicts a person walking across the frame, perpendicular to the camera (person closer to camera); and,
Column (c) depicts a person walking away and across from the camera, in a $45^{\circ}$ angle (person to the right).
Actions close to the centroids depict a common variation of the action in hand, in this case, the walking direction.
} % \small
} % \caption
\label{supp_basewords_fine}
% \vspace{-0.2cm}
\end{figure}
